# Supplementary material for: Towards Pair Atomic Density Fitting for Correlation Energies with Benchmark Accuracy
Source: arXiv:2211.16310 ancillary file (2022-11-29)
Supplement: Supplementary file 1 [file si.pdf]

# Supporting information to: Towards Pair Atomic Density Fitting for Correlation Energies with Benchmark Accuracy.

Edoardo Spadetto,*,† Pier Herman Theodoor Philipsen,*,† Arno Förster,*,† and Lucas Visscher‡

†*Software for Chemistry and Materials NV, NL, 1081HV, Amsterdam, The Netherlands*

‡*Theoretical Chemistry, Vrije Universiteit, De Boelelaan 1083, NL-1081 HV, Amsterdam, The Netherlands*

E-mail: spadetto@scm.com; philipsen@scm.com; foerster@scm.com

## 1 Basis set convergence for CIM8 Set

We here list the non-covalent interaction energies of the molecules in the Cim8 for different basis sets and different extrapolation schemes, calculated with and without counterpoise corrections.

Table 1: Interaction energies calculated with different basis sets and extrapolation schemes for the first molecule in the CIM8 set, "Capsule" with and without counterpoise corrections. $\Delta$ denotes the difference between the corrected and the non-corrected results. All values are in kcal/mol.

| cp correction [%] | DZ | TZ | QZ | (D,T) | (T,Q) |
|---|---|---|---|---|---|
| 100 | −39.86 | −52.51 | −60.17 | −58.22 | −64.86 |
| 0 | −70.50 | −66.08 | −53.44 | −67.80 | −56.93 |
| $\Delta$ | 30.64 | 13.58 | −6.73 | 9.58 | −7.93 |

Table 2: Interaction energies calculated with different basis sets and the corresponding extrapolated results for all molecules in the CIM8 set with and without counterpoise corrections. All values are in kcal/mol.

| | 100 % cp | | | 0 % cp | | |
|---|---|---|---|---|---|---|
| System | DZ | TZ | (D,T) | DZ | TZ | (D,T) |
| 1 | −39.86 | −52.51 | −58.22 | −70.50 | −66.08 | −67.80 |
| 2 | −30.26 | −47.76 | −55.76 | −75.49 | −62.15 | −62.79 |
| 3 | −23.46 | −28.29 | −31.01 | −40.74 | −34.46 | −34.67 |
| 4 | −8.91 | −12.67 | −14.09 | −15.10 | −20.91 | −24.90 |
| 5 | −18.10 | −29.40 | −34.31 | −39.93 | −43.65 | −48.67 |
| 6 | −21.39 | −47.42 | −58.97 | −86.19 | −79.77 | −86.81 |
| 7 | −254.48 | −306.17 | −336.83 | −390.89 | −391.67 | −414.75 |
| 8 | −6.47 | −19.94 | −25.58 | −29.43 | −35.45 | −41.27 |

# 2 Settings

Settings needed to reproduce our results are shown in 3 through BAND input files. The used development version includes new keywords which are expected to be kept in the new release version. The keyword `Method FromBasisProducts` switches on the fit set algorithm described in the main text. `OneCenterDependencyThreshold` is the $\epsilon_{\text{fit}}$ threshold, and finally `boostL` enables the $l$-e method. To enable Löwdin orthonormalization we use the `dependency` block with keyword `allowbasisdependency` which, if not present, leads to a stop of the calculation if unsafe linear dependencies are present in the basis set. In the same block it is possible to specify $\epsilon_{\text{bas}}$ through the `bas` keyword. In ADF, the same new keywords have been introduced as can be seen in table 4.

# 3 Reduced fit quality for $5\zeta$

In table 5 we list molecules for which $5\zeta$ simulation needed a lower fit quality. This was necessary to overcome the memory large consumption during generation of the fit functions.

Table 3: BAND settings when compared with Psi4, `boostL` that is $l$-e is set to true only for `CC-TZPGTO`. `CC-XZPGTO` are exactly the Dunnings correlation consistent basis sets, cc-PVXZ. The Slater basis `TZ2PSTO` is equal to `TZ2P` in ADF. `OneCenterDependencyThreshold` i.e. $\epsilon_{\text{fit}}$ is always set equal to $10^{-12}$ except for some large molecules which for computational reasons it is set to $10^{-10}$. These molecules are listed in table 5. The keyword `bas` by default is set to $10^{-8}$

```
Engine BAND
  Basis
    Core None
    Type CC-TZPGTO ( or CC-QZPGTO, CC-5ZPGTO, TZ2PSTO )
  End
  MBPT
    dependency TRUE
  End
  NumericalQuality VeryGood
  RIHartreeFock
    DependencyCoreRange 0.0
    DependencyThreshold 1e-3
    FitGenerationDetails
      Method FromBasisProducts
      OneCenterDependencyThreshold 1e-12 (1e-10)
      boostL True (or False)
    End
    FitSetQuality VeryGood
  End
  Relativity
    Level None
  End
  SoftConfinement
    Quality Excellent
  End
  XC
    HartreeFock
    MP2
  End
  dependency
    AllowBasisDependency
    (bas 1e-4)
  End
EndEngine
```

Table 4: Settings of ADF compared with BAND

```
Engine ADF
  Basis
    Core None
    Type TZ2P
  End
  MBPT
    dependency True
  End
  NumericalQuality VeryGood
  RIHartreeFock
    DependencyCoreRange 0.0
    DependencyThreshold 1e-3
    FitGenerationDetails
      OneCenterDependencyThreshold 1e-12
    End
    FitSetQuality FromBasisProducts
  End
  XC
    MP2
  End
  symmetry nosym
EndEngine
```

Table 5: Molecules for which cc-PV5Z fit set had quality $\epsilon_{\text{fit}} = 10^{-10}$ instead of $10^{-12}$

| Index | Molecule |
|---|---|
| 43 | UracilNeopentane |
| 35 | NeopentanePentane |
| 37 | CyclopentaneNeopentane |
| 35 | NeopentanePentane |
| 41 | UracilPentane |
| 34 | PentanePentane |
| 37 | CyclopentaneNeopentane |
